# Supplementary material for: VisualAgentBench: Towards Large Multimodal Models as Visual Foundation Agents
Source: arXiv:2408.06327 source file (2024-08-12)
Supplement: Supplementary file 1 [file evaluation_details.tex]

\section{More Experimental Results \& Analysis}
\label{app:exp_details}

\subsection{On the multi-task fine-tuning on \sm}
Despite existing research such as AgentTuning~\cite{zeng2023agenttuning} and AgentLumos~\cite{yin2023lumos} indicating that increasing the variety of training data types can improve agent performance, we find that when task properties are disparate, using a combined training set can actually harm performance (Table~\ref{tab:training}).
\begin{table}[t]
\centering
\caption{Comparing multitask (the main setting) and task-specific fine-tuning on \sm of CogVLM2. }
\vspace{1mm}

\resizebox{\columnwidth}{!}{
\begin{tabular}{@{}lcccccc@{}}
\toprule
\multirow{2}{*}{Method}            & \multirow{2}{*}{\begin{tabular}[c]{@{}c@{}}Overall\\ SR\end{tabular}} & \multicolumn{2}{c}{Embodied}                & \multicolumn{2}{c}{GUI} & Visual Design \\ \cmidrule(l){3-4} \cmidrule(l){5-6} \cmidrule(l){7-7} 
                                   &                                                                       & OmniGibson          & Minecraft           & Mobile  & WebArena-Lite & CSS           \\ \midrule
\texttt{CogVLM2} -task-specific FT & \textbf{\num{12.8}}                                                                  & \textbf{\num{6.6}}                  & \textbf{\num{25.9}}                 & \textbf{\num{12.6}}    & \textbf{\num{4.2}}           & \num{14.5}          \\
\qquad\qquad -multitask FT               & \num{10.3}                                                                   & \num{3.3} & \textbf{\num{25.9}} & \num{1.7}    & \num{3.0}           & \textbf{\num{17.6}}           \\ \bottomrule
\end{tabular}
\label{tab:training}
}
\end{table}
